# Supplementary material for: Diagnostic Benchmark and Iterative Inpainting for Layout-Guided Image Generation
Source: arXiv:2304.06671 source file (2024-07-21)
Supplement: Supplementary file 1 [file intermediate_steps_example_additional.tex]

\begin{table*}[t]
\begin{center}
    \resizebox{\linewidth}{!}{
      
        \begin{tabular}{l | c c c c c c c c c c c c c | c}
          \toprule

          Update & \multicolumn{13}{c |}{{\large  Intermediate Generation}}
          & {\large  GT image} \\
          \midrule

        & Step 1 & Step 2 & Step 3 & Step 4 & Step 5 & Step 6 & Step 7 & Step 8 & Step 9 & Step 10 & Step 11 & Step 12 & Step 13 \\
            Prompts & 
            Add red metal cube &
            Add purple metal sphere &
            Add cyan metal cube &
            Add gray metal cube &
            Add brown rubber cube &
            Add blue rubber cube &
            Add purple rubber cube &
            Add purple metal cube &
            Add gray metal cylinder &
            Add yellow rubber cylinder &
            Add gray rubber cylinder &
            Add red rubber cylinder &
            Add gray background \\
          \midrule
        \makecell[l]{Crop\&Paste \\ (default)}
          & \adjustbox{valign=c}{\includegraphics[height=0.1\textwidth]{images/intermediate_generation/LayoutBench_val_number_11-13_001680/0_generated.png}} &
          \adjustbox{valign=c}{\includegraphics[height=0.1\textwidth]{images/intermediate_generation/LayoutBench_val_number_11-13_001680/1_generated.png}} &
          \adjustbox{valign=c}{\includegraphics[height=0.1\textwidth]{images/intermediate_generation/LayoutBench_val_number_11-13_001680/2_generated.png}} &
          \adjustbox{valign=c}{\includegraphics[height=0.1\textwidth]{images/intermediate_generation/LayoutBench_val_number_11-13_001680/3_generated.png}} &
          \adjustbox{valign=c}{\includegraphics[height=0.1\textwidth]{images/intermediate_generation/LayoutBench_val_number_11-13_001680/4_generated.png}} &
          \adjustbox{valign=c}{\includegraphics[height=0.1\textwidth]{images/intermediate_generation/LayoutBench_val_number_11-13_001680/5_generated.png}} &
          \adjustbox{valign=c}{\includegraphics[height=0.1\textwidth]{images/intermediate_generation/LayoutBench_val_number_11-13_001680/6_generated.png}} &
          \adjustbox{valign=c}{\includegraphics[height=0.1\textwidth]{images/intermediate_generation/LayoutBench_val_number_11-13_001680/7_generated.png}} &
          \adjustbox{valign=c}{\includegraphics[height=0.1\textwidth]{images/intermediate_generation/LayoutBench_val_number_11-13_001680/8_generated.png}} &
          \adjustbox{valign=c}{\includegraphics[height=0.1\textwidth]{images/intermediate_generation/LayoutBench_val_number_11-13_001680/9_generated.png}} &
          \adjustbox{valign=c}{\includegraphics[height=0.1\textwidth]{images/intermediate_generation/LayoutBench_val_number_11-13_001680/10_generated.png}} &
          \adjustbox{valign=c}{\includegraphics[height=0.1\textwidth]{images/intermediate_generation/LayoutBench_val_number_11-13_001680/11_generated.png}} &
          \adjustbox{valign=c}{\includegraphics[height=0.1\textwidth]{images/intermediate_generation/LayoutBench_val_number_11-13_001680/12_generated.png}} &
          \adjustbox{valign=c}{\includegraphics[height=0.1\textwidth]{images/intermediate_generation/LayoutBench_val_number_11-13_001680.png}} \\
          \midrule
          Repaint &
            \adjustbox{valign=c}{\includegraphics[height=0.1\textwidth]{images/intermediate_generation/Nopaste_LayoutBench_val_number_11-13_001680/0_generated.png}} &
            \adjustbox{valign=c}{\includegraphics[height=0.1\textwidth]{images/intermediate_generation/Nopaste_LayoutBench_val_number_11-13_001680/1_generated.png}} &
            \adjustbox{valign=c}{\includegraphics[height=0.1\textwidth]{images/intermediate_generation/Nopaste_LayoutBench_val_number_11-13_001680/2_generated.png}} &
            \adjustbox{valign=c}{\includegraphics[height=0.1\textwidth]{images/intermediate_generation/Nopaste_LayoutBench_val_number_11-13_001680/3_generated.png}} &
            \adjustbox{valign=c}{\includegraphics[height=0.1\textwidth]{images/intermediate_generation/Nopaste_LayoutBench_val_number_11-13_001680/4_generated.png}} &
            \adjustbox{valign=c}{\includegraphics[height=0.1\textwidth]{images/intermediate_generation/Nopaste_LayoutBench_val_number_11-13_001680/5_generated.png}} &
            \adjustbox{valign=c}{\includegraphics[height=0.1\textwidth]{images/intermediate_generation/Nopaste_LayoutBench_val_number_11-13_001680/6_generated.png}} &
            \adjustbox{valign=c}{\includegraphics[height=0.1\textwidth]{images/intermediate_generation/Nopaste_LayoutBench_val_number_11-13_001680/7_generated.png}} &
            \adjustbox{valign=c}{\includegraphics[height=0.1\textwidth]{images/intermediate_generation/Nopaste_LayoutBench_val_number_11-13_001680/8_generated.png}} &
            \adjustbox{valign=c}{\includegraphics[height=0.1\textwidth]{images/intermediate_generation/Nopaste_LayoutBench_val_number_11-13_001680/9_generated.png}} &
            \adjustbox{valign=c}{\includegraphics[height=0.1\textwidth]{images/intermediate_generation/Nopaste_LayoutBench_val_number_11-13_001680/10_generated.png}} &
            \adjustbox{valign=c}{\includegraphics[height=0.1\textwidth]{images/intermediate_generation/Nopaste_LayoutBench_val_number_11-13_001680/11_generated.png}} &
            \adjustbox{valign=c}{\includegraphics[height=0.1\textwidth]{images/intermediate_generation/Nopaste_LayoutBench_val_number_11-13_001680/12_generated.png}} &
            \adjustbox{valign=c}{\includegraphics[height=0.1\textwidth]{images/intermediate_generation/LayoutBench_val_number_11-13_001680.png}} \\
          \bottomrule
      \end{tabular}
    }
\end{center}
\caption{
Additional intermediate generation samples of \method{}.
}
\label{tab:intermediate_generation_samples_addtional}
\end{table*}
